# Supplementary material for: Revisiting Fully Convolutional Geometric Features for Object 6D Pose Estimation
Source: arXiv:2307.15514 source file (2023-10-03)
Supplement: Supplementary file 2 [file mycommands.tex]

% Acronym

% LMO colors
\definecolor{ape}{RGB}{143,24,24}
\definecolor{can}{RGB}{237,154,59}
\definecolor{cat}{RGB}{145,70,163}
\definecolor{driller}{RGB}{57,67,53}
\definecolor{duck}{RGB}{226,215,62}
\definecolor{eggbox}{RGB}{111,161,18}
\definecolor{glue}{RGB}{150,141,137}
\definecolor{holepuncher}{RGB}{46,54,110}
