# Supplementary material for: Revisiting Fully Convolutional Geometric Features for Object 6D Pose Estimation
Source: arXiv:2307.15514 source file (2023-10-03)
Supplement: Supplementary file 3 [file mypackages.tex]

\usepackage{booktabs}
\usepackage{multirow}
\usepackage{multicol}

\usepackage{pifont}

\usepackage{enumitem}
\usepackage{microtype}
\usepackage{subcaption}
\usepackage{flushend}

\usepackage{balance}

\usepackage{contour}
\contourlength{0.33pt}

\usepackage{pgf,tikz}
\usetikzlibrary{shapes.geometric}
\usepackage{pgfplots}
\usepackage{filecontents}
\pgfplotsset{compat=1.7}
\newlength\figureheight
\newlength\figurewidth

\usepackage{soul}

\usepackage[permil]{overpic}

\usepackage{todonotes}

\usepackage{wrapfig}
